# Supplementary material for: Estimation of end-of-outbreak probabilities in the presence of delayed and incomplete case reporting
Source: arXiv:2409.16531 source file (2024-11-24)
Supplement: Supplementary file 1 [file supp.pdf]

# Estimation of end-of-outbreak probabilities in the presence of delayed and incomplete case reporting

## Supplementary Material

### S1 Derivation of alternative definitions of end-of-outbreak probability

#### Probability of no future infections or case notification

The probability that there are no infections and no case notifications on or after day  $t$  may be expressed

$$P(\text{no future infections or notifications}) = P(\text{no future infections}) P(\text{no future notifications} \mid \text{no future infections}) \quad (\text{S1})$$

The first probability on the right-hand side of Eq. (S1) is equal to  $P_0 = e^{-R\gamma t}$  by definition. The second probability, which we denote  $\phi_t$ , may be expressed as

$$\phi_t = \prod_{t'=t}^{\infty} P(C_{t'} = 0 \mid I_s = 0 \forall s \geq t) \quad (\text{S2})$$

Given  $Z_{st'}$  (i.e. the number of individuals who were infected on day  $s$  and with a notification date on day  $t'$ , as defined in Eq. (4) of the main article) for  $s < t$ , the random variables  $(C_{t'} \mid I_s = 0 \forall s \geq t)$  are conditionally independent negative binomial random variables with mean  $\alpha \sum_{s=1}^{t-1} Z_{st'}$  and dispersion parameter  $k_c$ . Thus, we have the following expression for  $\phi_t$ :

$$\phi_t = \prod_{t'=t}^{\infty} \left( \frac{k_c}{k_c + \alpha \sum_{s=1}^{t-1} Z_{st'}} \right)^{k_c}. \quad (\text{S3})$$

In the limiting case  $k_c \rightarrow \infty$  (i.e. the number of daily case notifications is Poisson distributed),  $\phi_t$  is given by

$$\phi_t = \prod_{t'=t}^{\infty} e^{-\alpha \sum_{s=1}^{t-1} Z_{st'}}. \quad (\text{S4})$$

### Probability of ultimate extinction

Let  $q \in [0, 1]$  denote the probability of ultimate extinction (PUE) for an outbreak seeded with a random fully infectious individual. Now consider an individual  $i$  who was infected at time  $t - s$  and has a given individual transmission multiplier  $y_i$ . Let the random variable  $X_i$  be the total number of people infected by that individual after time  $t$ . The probability  $p_i$  that the transmission tree starting from individual  $i$  eventually goes extinct is

$$p_i = \sum_n P(X_i = n) q^n \quad (\text{S5})$$

This is equivalent to  $p = G_i(q)$  where  $G_i$  is the generating function for  $X_i$ .

If the reproduction number after time  $t$  is equal to a constant  $R$ , then  $X_i$  is a Poisson random variable with mean  $Ry_i(1 - F_{s-1})$ . Since the generating function for a Poisson random variable with mean  $\lambda$  is  $G(z) = e^{-\lambda(1-z)}$ , we have

$$p_i = e^{-Ry_i(1-F_{s-1})(1-q)} \quad (\text{S6})$$

Now suppose instead of one previous infection, there was a time series of daily infections  $I_{t-s}$ . The probability that the transmission trees starting from all  $N$  previous infections independently go extinct is

$$\text{PUE} = \prod_{i=1}^N p_i = \exp \left( -R(1-q) \sum_{s=1}^{t-1} (1 - F_{s-1}) \sum_{j=1}^{I_{t-s}} y_{t-s,j} \right) \quad (\text{S7})$$

where  $y_{t-s,j}$  denotes the transmission multiplier for the  $j^{\text{th}}$  person infected on day  $t - s$ . By definition,  $\sum_{j=1}^{I_{t-s}} y_{t-s,j}$  is equal to  $Y_{t-s}$  so we have

$$\text{PUE} = e^{-R(1-q)\gamma_t} \quad (\text{S8})$$

where  $\gamma_t$  is as defined in Eq. (7) of the main article.

The value of  $q$  is the solution of the equation  $q = H(q)$  where  $H$  is the probability generating function (PGF) of the offspring distribution, which is negative binomial with mean  $R$  and dispersion parameter  $k_r$ . Hence, for finite values of  $k_r$ ,  $q$  satisfies

$$q = H(q) = \left( \frac{k_r}{k_r + R(1-q)} \right)_r^k, \quad (\text{S9})$$

which is straightforward to solve numerically for given values of  $R$  and  $k_r$ . In the limiting case  $k_r \rightarrow \infty$  where the offspring distribution is Poisson with mean  $R$ ,  $q$  satisfies

$$q = H(q) = e^{-R(1-q)}. \quad (\text{S10})$$

Note  $H$  differs from  $G_i$  because  $H$  is the PGF for the offspring distribution across all individuals, which is negative binomial, whereas  $G_i$  is the PGF of the offspring distribution of an individual with a specific transmission multiplier  $y_i$  (restricted to times  $t > s$  after infection), which is Poisson with mean proportional to  $y_i$ .

## S2 Supplementary results and sensitivity analysis

Figures S1–S3 provide supplementary results for the New Zealand Covid-19 outbreak, showing the estimated time-varying reproduction number  $R_t$ , number of daily new local infections  $I_t$ , daily local reported cases  $C_t$ , and probability of  $P_0$  of no future infections. Figure S1 shows results for different values of the case notification probability  $\alpha$  and the mean time  $t_n$  from infection to notification. These results supplement those in Figure 2 of the main article. Figure S2 shows results for different values of the dispersion parameter  $k_r$ , corresponding to different levels of individual heterogeneity in transmission probabilities. These results supplement those in Figure 3 of the main article. Figure S3 shows the results of a sensitivity analysis for the random walk parameters  $\sigma_R$  and  $\delta_C$  that govern the prior for the reproduction number  $R_t$ . Figures S4–S6 show corresponding supplementary results for the DRC EVD outbreak.

The sensitivity analysis on the standard deviation  $\sigma_R$  in the daily change in  $R_t$  and the expected daily change  $\delta_c$  in  $R_t$  at the beginning of the intervention (Figures S3 and S6) shows that the main results are not highly sensitive to the chosen parameter values. The role of these parameters is to specify the prior distribution for the time-varying reproduction number  $R_t$ .

Figures S1–S6 also explore the variability amongst particles in the estimated probability  $P_0$  of no future infections, indicated by the shaded blue band corresponding to the 5th and 95th percentiles of  $P_0$  across the  $m = 10^5$  particles. These results show that the value of  $P_0$  can vary quite widely across particles: for some time points the shaded interval encompasses almost the whole of  $[0, 1]$ . However, as we explain in the following paragraph, these results need to be interpreted with caution and do not mean that the model provides no information on the value of  $P_0$ .

The uncertainty in the outcome of interest (no future infections on or after day  $t$ ) can be decomposed into two parts: (1) uncertainty about the history and current state of the epidemic process given data up to time  $t$  (i.e. about the values of the hidden states  $R_{t'}$  and  $I_{t'}$  for  $0 \leq t' \leq t$ ); and (2) uncertainty about the future epidemic trajectory for given values of  $R_{t'}$  and  $I_{t'}$  for  $0 \leq t' \leq t$ . These two sources of uncertainty are handled by the model in

different ways. Source (1) is handled by stochastic simulation of  $m$  particles: at time  $t$ , each particle represents a sample from the approximate posterior distribution over the hidden states  $R_{t'}$  and  $I_{t'}$  for  $0 \leq t' \leq t$ , given data on reported cases  $C_{t'}$  for  $0 \leq t' \leq t$ . Source (2) is handled by analytically calculating the probability  $P_0$  (via Eq. (6) of the main article) for each particle, as a function of that particle's values for  $I_{t'}$  for  $0 \leq t' \leq t$ . The observation that  $P_0$  sometimes varies widely amongst particles simply shows that source (1) is a major contributor to the overall uncertainty. This is not a surprising result, but does illustrate the importance of accounting for uncertainty in both previous and future epidemic dynamics. We emphasise that our overall  $P_0$  estimates (i.e. the average across particles) integrate both sources of uncertainty in the probability of future cases.

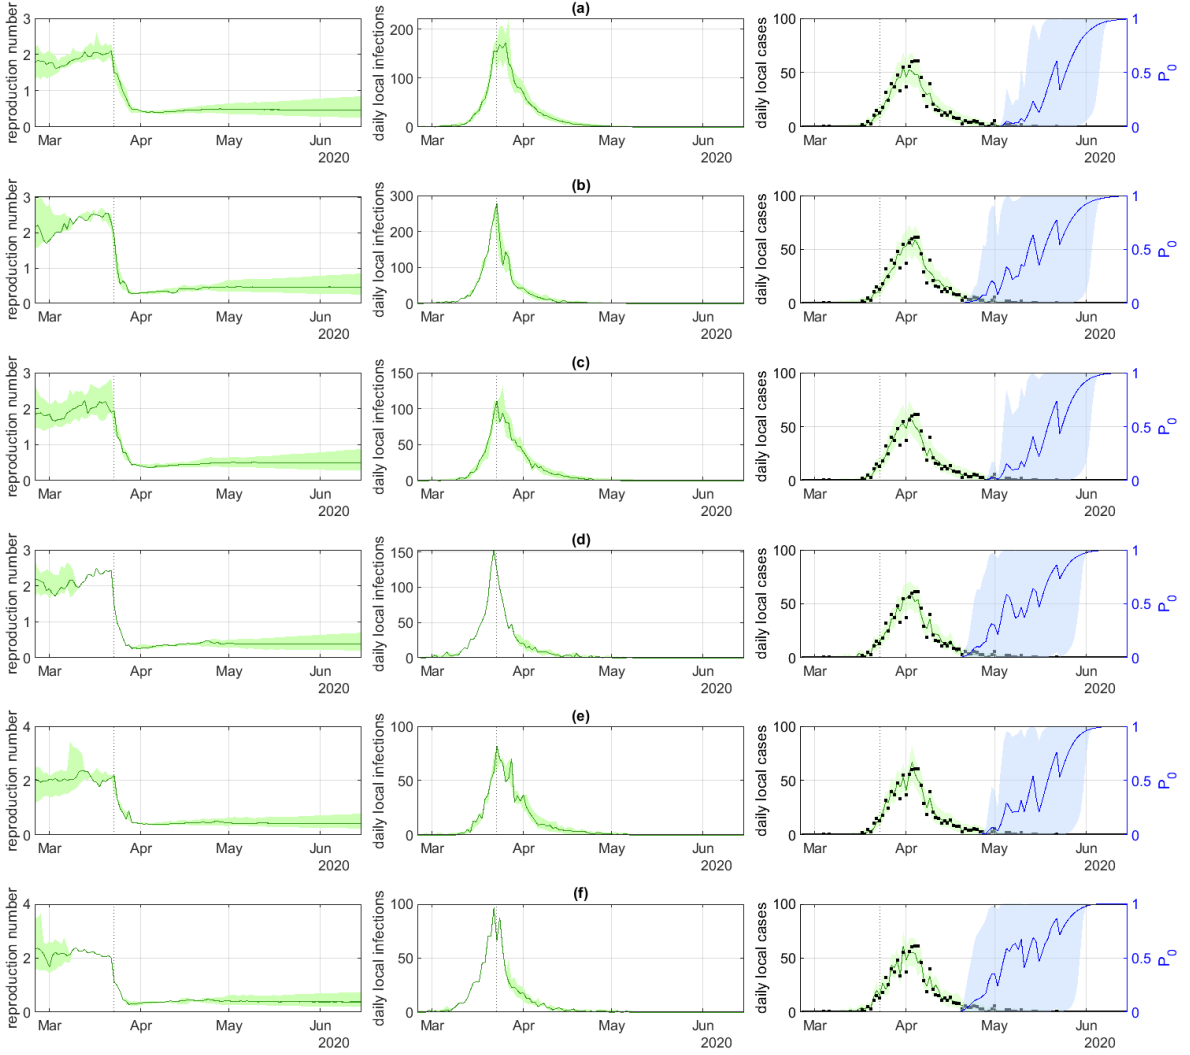

Figure S1: Model results for the New Zealand Covid-19 outbreak for different values of the notification probability  $\alpha$  and mean time from infection to notification  $t_n$ . Notification probability in (a,b)  $\alpha = 0.4$ ; in (c,d)  $\alpha = 0.7$ ; in (e,f)  $\alpha = 1$ . Mean time from infection to notification in (a,c,e)  $t_n = 7.7$  days; in (b,d,f)  $t_n = 11.2$  days. For each row of graphs, the left-hand plot shows the instantaneous reproduction number  $R_t$ , the central plot shows daily new local infections  $I_t$ , and the right-hand plot shows daily local case notifications  $C_t$  (green) and probability  $P_0$  of no future infections (blue). Solid curves show the median and shaded bands shows the 5th and 95th percentiles of  $m = 10^5$  particles. Black points show data for daily local case notifications. Dotted vertical line shows the start of the 7-day time window in which a rapid drop in the reproduction number was expected *a priori*. Dispersion parameter  $k_r = \infty$  (i.e. offspring distribution was Poisson).

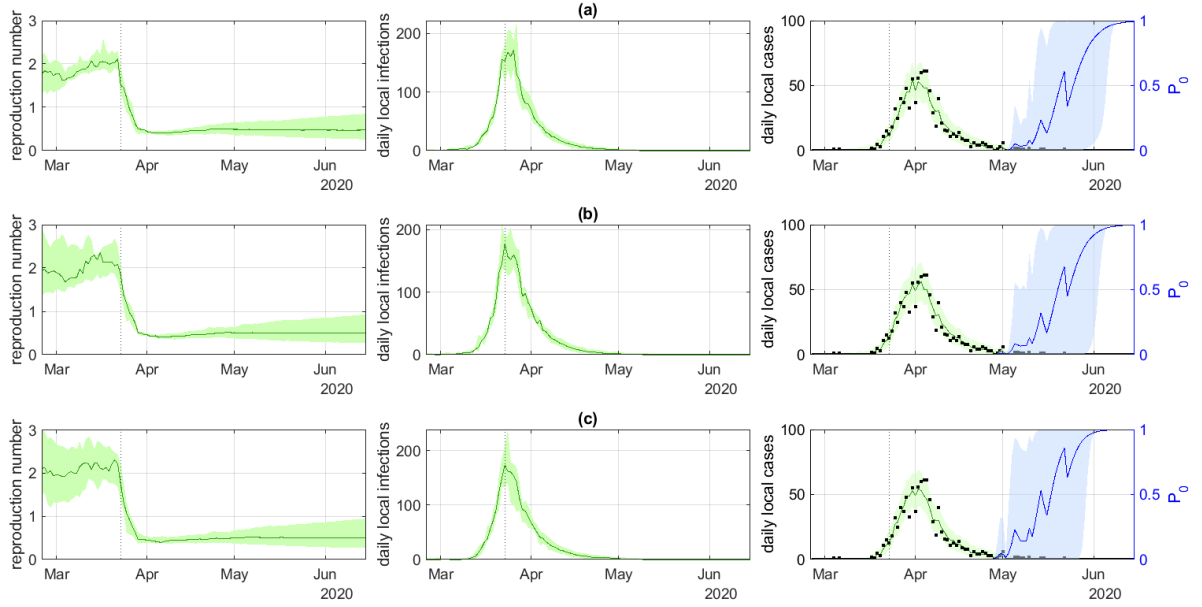

Figure S2: Model results for the New Zealand Covid-19 outbreak for different values of the dispersion parameter: (a)  $k_r = \infty$  (i.e. offspring distribution was Poisson); (b)  $k_r = 1$ ; (c)  $k_r = 0.2$ . For each row of graphs, the left-hand plot shows the instantaneous reproduction number  $R_t$ , the central plot shows daily new local infections  $I_t$ , and the right-hand plot shows daily local case notifications  $C_t$  (green) and probability  $P_0$  of no future infections (blue). Solid curves show the median and shaded bands shows the 5th and 95th percentiles of  $m = 10^5$  particles. Black points show data for daily local case notifications. Dotted vertical line shows the start of the 7-day time window in which a rapid drop in the reproduction number was expected *a priori*. Notification probability  $\alpha = 0.4$ ; mean time from infection to notification  $t_n = 7.7$  days.

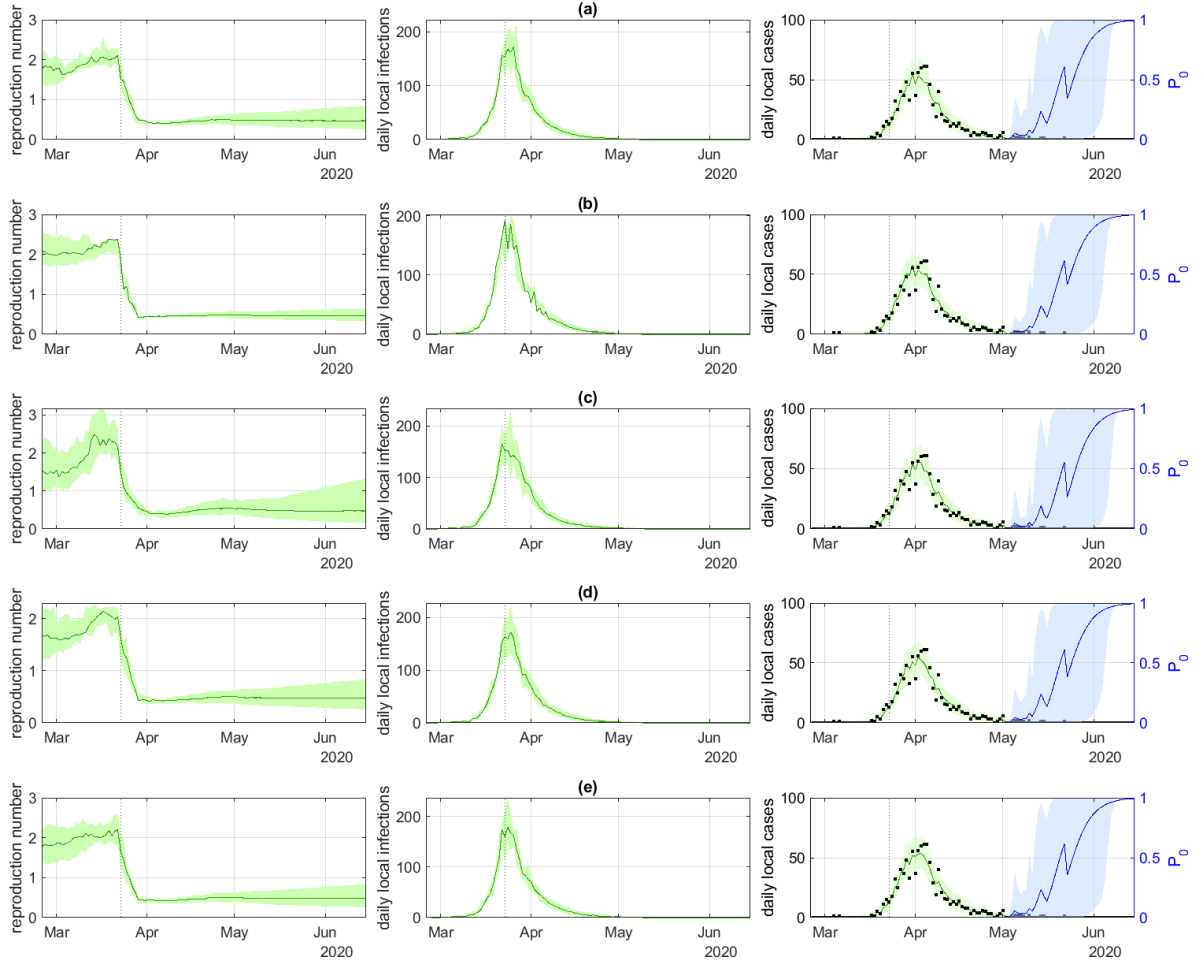

Figure S3: Model results for the New Zealand Covid-19 outbreak for different values of the random walk parameters  $\sigma_R$  and  $\delta_c$ : (a)  $\sigma_R = 0.05$ ,  $\delta_c = -0.1$ ; (b)  $\sigma_R = 0.025$ ,  $\delta_c = -0.1$ ; (c)  $\sigma_R = 0.1$ ,  $\delta_c = -0.1$ ; (d)  $\sigma_R = 0.05$ ,  $\delta_c = -0.05$ ; (e)  $\sigma_R = 0.05$ ,  $\delta_c = -0.2$ . For each row of graphs, the left-hand plot shows the instantaneous reproduction number  $R_t$ , the central plot shows daily new local infections  $I_t$ , and the right-hand plot shows daily local case notifications  $C_t$  (green) and probability  $P_0$  of no future infections (blue). Solid curves show the median and shaded bands shows the 5th and 95th percentiles of  $m = 10^5$  particles. Black points show data for daily local case notifications. Dotted vertical line shows the start of the 7-day time window in which a rapid drop in the reproduction number was expected *a priori*. Notification probability  $\alpha = 0.4$ ; mean time from infection to notification  $t_n = 7.7$  days; dispersion parameter  $k_r = \infty$  (i.e. offspring distribution was Poisson).

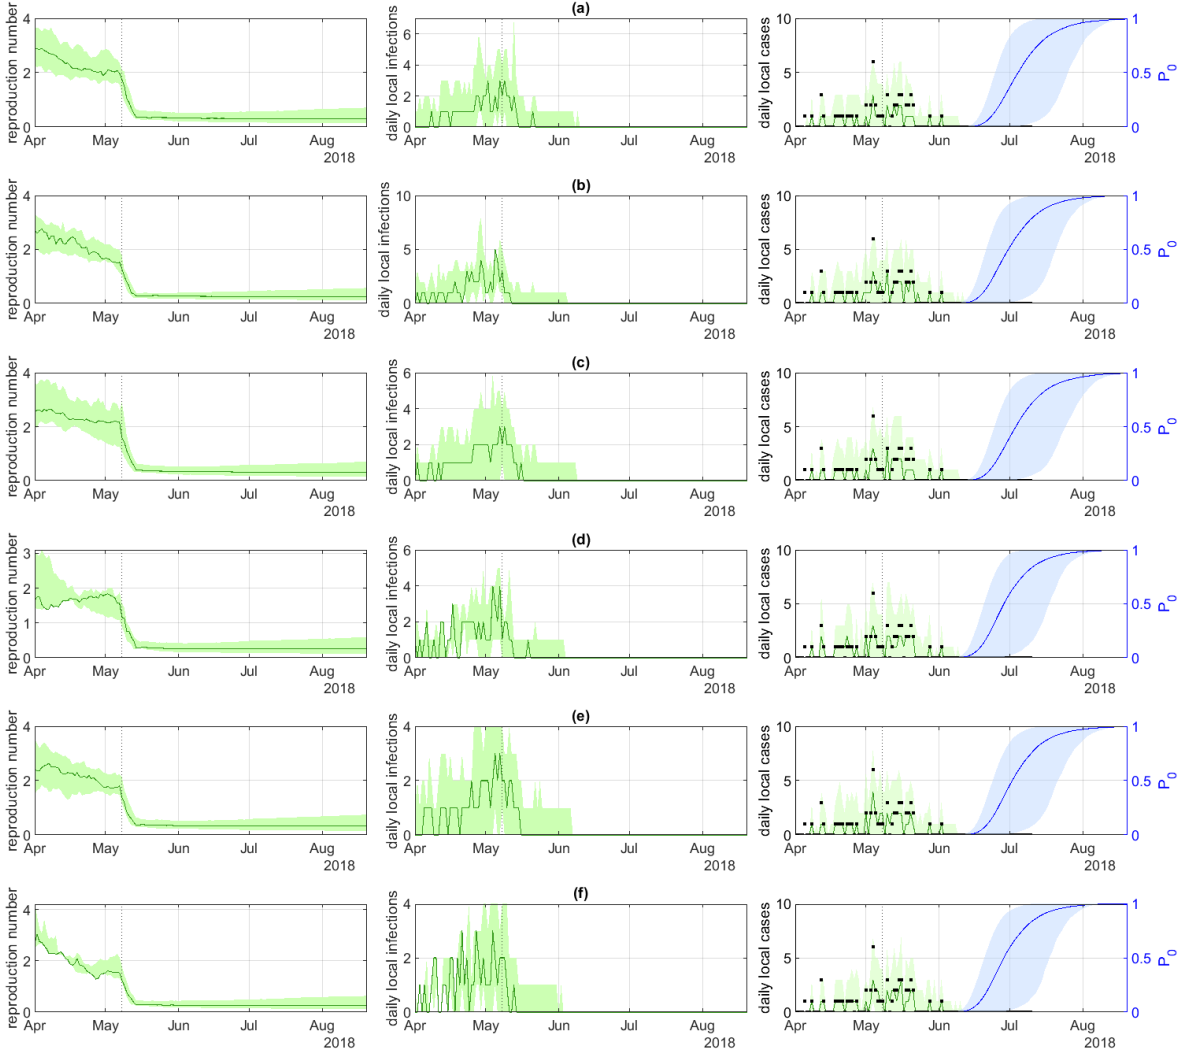

Figure S4: Model results for the DRC EVD outbreak for different values of the notification probability  $\alpha$  and mean time from infection to notification  $t_n$ . Notification probability in (a,b)  $\alpha = 0.8$ ; in (c,d)  $\alpha = 0.9$ ; in (e,f)  $\alpha = 1$ . Mean time from infection to notification in (a,c,e)  $t_n = 6.2$  days; in (b,d,f)  $t_n = 11.2$  days. For each row of graphs, the left-hand plot shows the instantaneous reproduction number  $R_t$ , the central plot shows daily new local infections  $I_t$ , and the right-hand plot shows daily local case notifications  $C_t$  (green) and probability  $P_0$  of no future infections (blue). Solid curves show the median and shaded bands shows the 5th and 95th percentiles of  $m = 10^5$  particles. Black points show data for daily local case notifications. Dotted vertical line shows the start of the 7-day time window in which a rapid drop in the reproduction number was expected *a priori*. Dispersion parameter  $k_r = \infty$  (i.e. offspring distribution was Poisson).

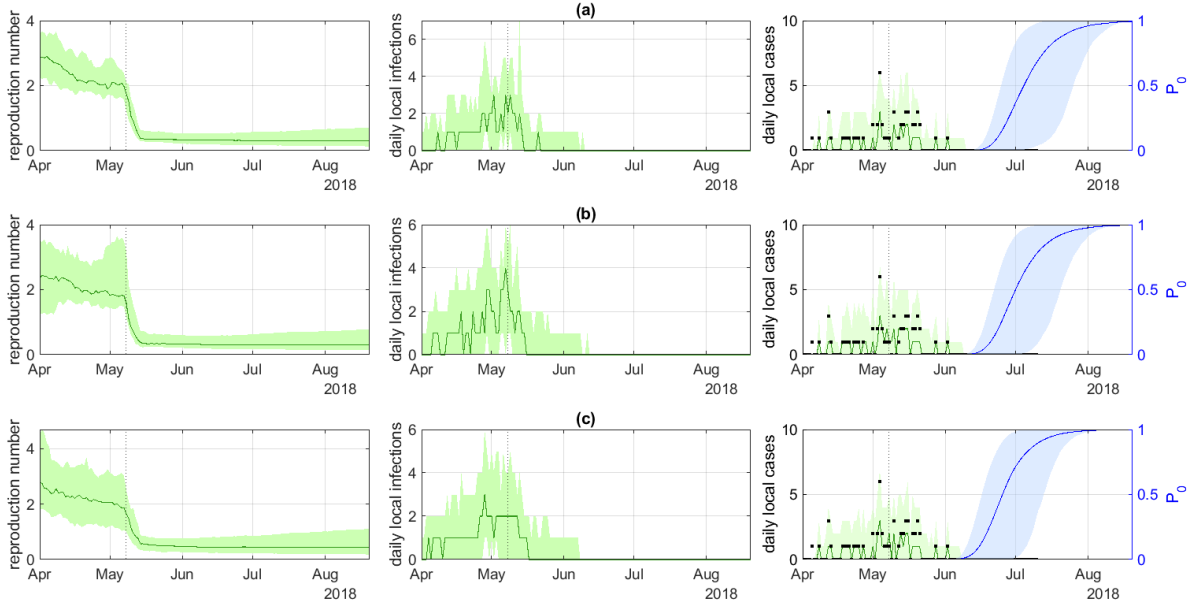

Figure S5: Model results for the DRC EVD outbreak for different values of the dispersion parameter: (a)  $k_r = \infty$  (i.e. offspring distribution was Poisson); (b)  $k_r = 1$ ; (c)  $k_r = 0.2$ . For each row of graphs, the left-hand plot shows the instantaneous reproduction number  $R_t$ , the central plot shows daily new local infections  $I_t$ , and the right-hand plot shows daily local case notifications  $C_t$  (green) and probability  $P_0$  of no future infections (blue). Solid curves show the median and shaded bands shows the 5th and 95th percentiles of  $m = 10^5$  particles. Black points show data for daily local case notifications. Dotted vertical line shows the start of the 7-day time window in which a rapid drop in the reproduction number was expected *a priori*. Notification probability  $\alpha = 0.4$ ; mean time from infection to notification  $t_n = 7.7$  days.

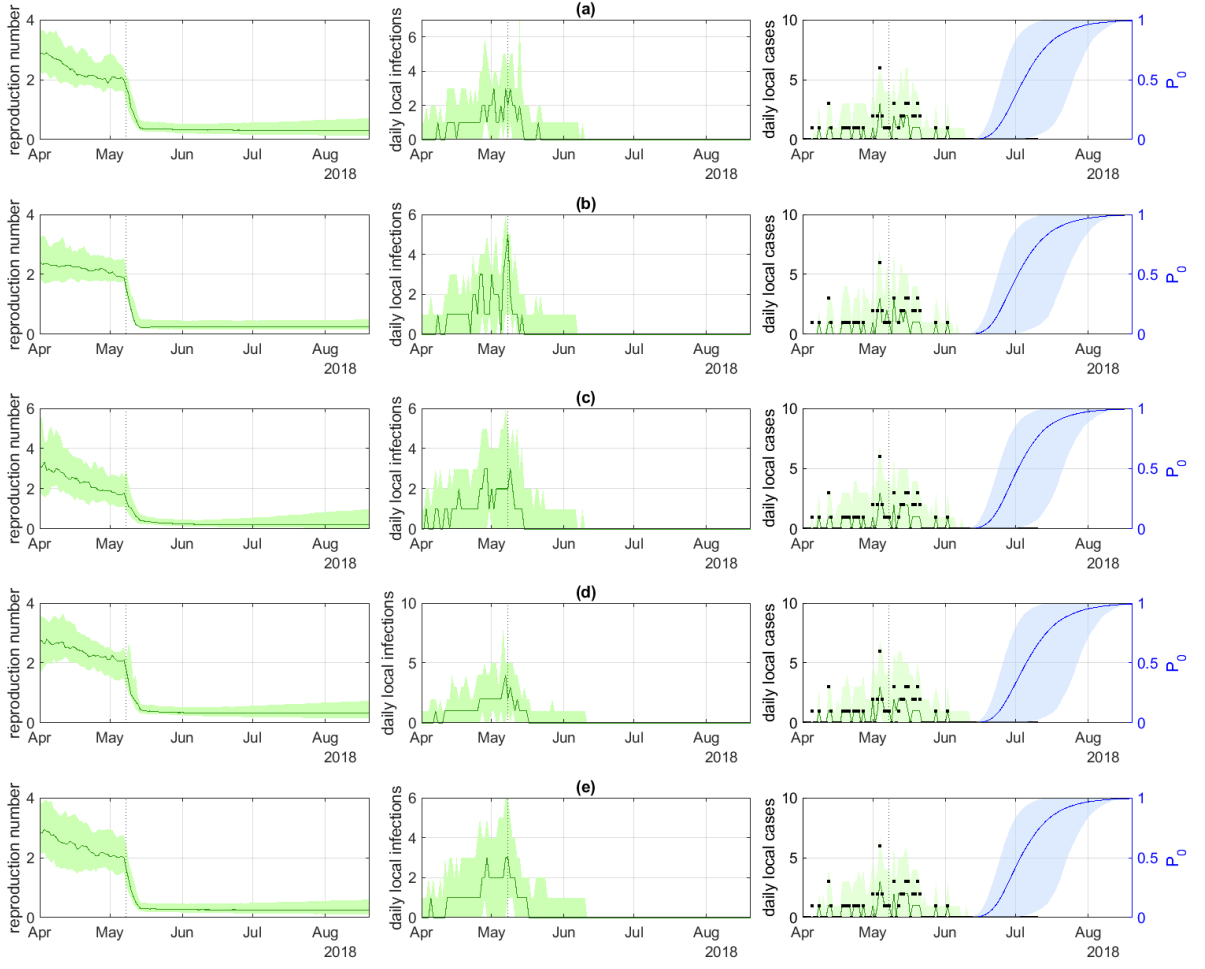

Figure S6: Model results for the DRC EVD outbreak for different values of the random walk parameters  $\sigma_R$  and  $\delta_c$ : (a)  $\sigma_R = 0.05$ ,  $\delta_c = -0.1$ ; (b)  $\sigma_R = 0.025$ ,  $\delta_c = -0.1$ ; (c)  $\sigma_R = 0.1$ ,  $\delta_c = -0.1$ ; (d)  $\sigma_R = 0.05$ ,  $\delta_c = -0.05$ ; (e)  $\sigma_R = 0.05$ ,  $\delta_c = -0.2$ . For each row of graphs, the left-hand plot shows the instantaneous reproduction number  $R_t$ , the central plot shows daily new local infections  $I_t$ , and the right-hand plot shows daily local case notifications  $C_t$  (green) and probability  $P_0$  of no future infections (blue). Solid curves show the median and shaded bands shows the 5th and 95th percentiles of  $m = 10^5$  particles. Black points show data for daily local case notifications. Dotted vertical line shows the start of the 7-day time window in which a rapid drop in the reproduction number was expected *a priori*. Notification probability  $\alpha = 0.8$ ; mean time from infection to notification  $t_n = 6.2$  days; dispersion parameter  $k_r = \infty$  (i.e. offspring distribution was Poisson).
